# Supplementary material for: Periodic motion of sedimenting flexible knots
Source: arXiv:1808.05818 ancillary file (2018-08-17)
Supplement: Supplementary file 1 [file Supplementary.pdf]

## Supplementary material for: "Periodic motion of sedimenting elastic knots"

Magdalena Gruziel<sup>1</sup>, Krishnan Thyagarajan<sup>2</sup>, Giovanni Dietler<sup>2</sup>,  
Andrzej Stasiak<sup>3,4</sup>, Maria L. Ekiel-Jeżewska<sup>1</sup>, and Piotr Szymczak<sup>5</sup>

<sup>1</sup>*Institute of Fundamental Technological Research,*

*Polish Academy of Sciences, Pawińskiego 5B, 02-106, Warsaw, Poland*

<sup>2</sup>*École Polytechnique Fédérale de Lausanne, Lab Phys Living Matter, CH-1015 Lausanne, Switzerland*

<sup>3</sup>*Center for Integrative Genomics, University of Lausanne, CH-1015 Lausanne, Switzerland*

<sup>4</sup>*SIB Swiss Institute of Bioinformatics, CH-1015, Lausanne, Switzerland and*

<sup>5</sup>*Institute of Theoretical Physics, Faculty of Physics,*

*University of Warsaw, Pasteura 5, 02-093, Warsaw, Poland*

### MOVIE CAPTIONS

- Movie 1:** Experiment: Settling of  $\mathcal{T}_{2,3}$  knot made of stainless steel chain in silicone oil. After initial phase the chain adopts a flat, extended configuration of two intertwined loops and performs an oscillatory swirling motions. There are about 5 swirls during the settling.
- Movie 2:** Experiment: Settling of stainless steel  $\mathcal{T}_{3,2}$  knot in silicone oil. The initial phase is slightly longer than in the case of  $\mathcal{T}_{2,3}$  but still the chain adopts an extended configuration and performs the swirling oscillations.
- Movie 3:** Experiment: Settling of stainless steel  $\mathcal{T}_{2,7}$  knot in silicone oil. The chain is the same length as in movies 1,2, so it is clearly more tightly knotted, but again adopts an extended horizontal configuration. In this case, one can also see, that the motion may be also viewed as a spinning of a circular screw.
- Movie 4:** Simulation: Settling of  $\mathcal{T}_{2,3}$  knot in a simulation with initial configuration given by Eq. (2) in the main article (i.e.  $\rho(\alpha) = r_0 + a \sin(q\alpha/p)$ ,  $z(\alpha) = a \cos(q\alpha/p)$ ) and  $N = 60$ . One can see here, that the swirling motion is accompanied by a slow, clockwise rotation of the system (about 30-40° during the whole movie).
- Movie 5:** Simulation: Settling of  $\mathcal{T}_{3,2}$  knot in a simulation with initial configuration given by Eq. (2) in the main article, with  $N = 90$ . Also in this case, the clockwise rotation of the system is visible (about 240°).
- Movie 6:** Simulation: Settling of  $\mathcal{T}_{2,7}$  knot in a simulation with initial configuration given by Eq. (2) in the main article, with  $N = 60$ . The clockwise rotation of the system (about 10-15°) is also visible.
- Movie 7:** Experiment: Settling of  $\mathcal{T}_{2,3}$  with one bead marked. This is a short part of Movie 1. By marking the bead, one can see that the rotation of the system is not observed at this short timescale. Also, clearly one sees the periodic swirling motion of the bead in  $\alpha$  direction.
- Movie 8:** Simulation: Settling of  $\mathcal{T}_{2,3}$  knot in a short simulation with initial configuration given by Eq. (2) in the main article, with  $N = 40$  and the Brownian motion included,  $Pe = 2$ . Although less regular, both the swirling motion, and the rotation are preserved even with the noise present in the system.

## DIMENSIONLESS PARAMETERS

One should note that, in contrast to the main text, throughout this SM all the parameters are dimensionless even though denoted by the same letters. Thus, all the dimensional length parameters ( $\rho, z, C$ ) will be divided by  $d$  and renamed, e.g.  $C/d \rightarrow C$ . Also the dimensional bending stiffness  $A$  defined in the main work, is now divided by  $F_0 d$ . With this, the value used in the main work would be simply  $A = 5$ .

## FITTING OF THE PARAMETERS

The fits, such as those presented in Fig. 4 in the main text or in Figs. 5–9 in this supplementary material, were performed separately for all three coordinates,  $\rho(t)$ ,  $\phi(t)$ , and  $z(t)$ . The parameter  $C$  in Eq. (4) of the main text can thus be obtained independently from these three fits. In Fig. 1 the resulting  $C$  is plotted for various values of  $N$ , various knot types,  $\mathcal{T}_{2,q}$ , and various  $A$  (only in the case of  $\mathcal{T}_{2,9}$ , for  $N=90,120$ ). In the ideal case, they should collapse on a single curve. The data in Fig. 1 shows that the three values converge to a single one with decreasing aspect ratio of the chains (i.e. increasing  $N$ ).

Another characteristics of the swirling motion is the velocity with which the crossing point between the strands propagates along the loop (defined as  $k = \rho_0 \tau_d / \tau_{swirl}$ ). This is shown in Fig. 2 for different knot types and  $N$ .

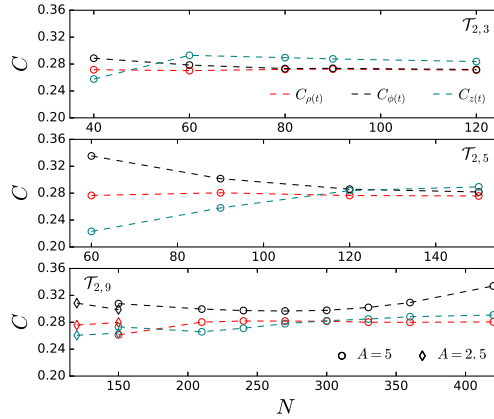

FIG. 1:  $C$  parameters (see Eq. (4) in the main text) obtained from the fit to  $\rho(t)$  (red),  $\phi(t)$  (blue), and  $z(t)$  (black) plotted against chain size,  $N$ , for various knots. For a  $\mathcal{T}_{2,9}$  knot also smaller bending stiffness was tested (results plotted with diamonds).

## OTHER KNOTS: $\mathcal{T}_{3,2}$

The  $\mathcal{T}_{3,2}$  knots were far less stable but still there was a well-defined frequency characterizing the motion (*cf.* Fig. 4). Fig. 3 presents snapshots from experiments (left) and simulations (right) showing the similarity of the configurations.

The time-dependent, scaled cylindrical coordinates of one of the beads  $\tilde{\rho}, \tilde{\alpha}, \tilde{z}$  (see main text) are presented in Fig. 4. Although the fitted sinusoids capture the swirling frequency quite well, the motion itself is much more complex and diverges from the simple approximation given by Eq. (4) in the main text.

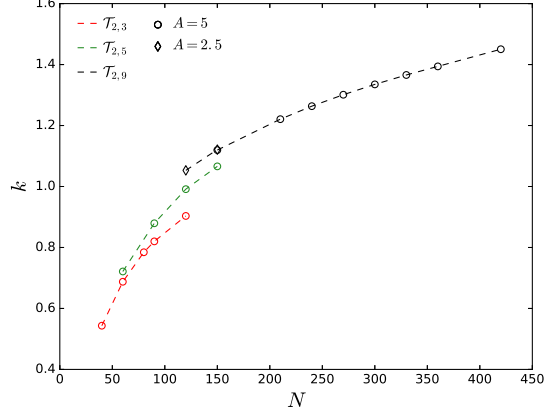

FIG. 2: The velocity ( $k = \rho_0 \tau_d / \tau_{swirl}$ ) with which the crossing point between the strands propagates along the loop, with  $\tau_{swirl}$  obtained by fitting the simulation data.

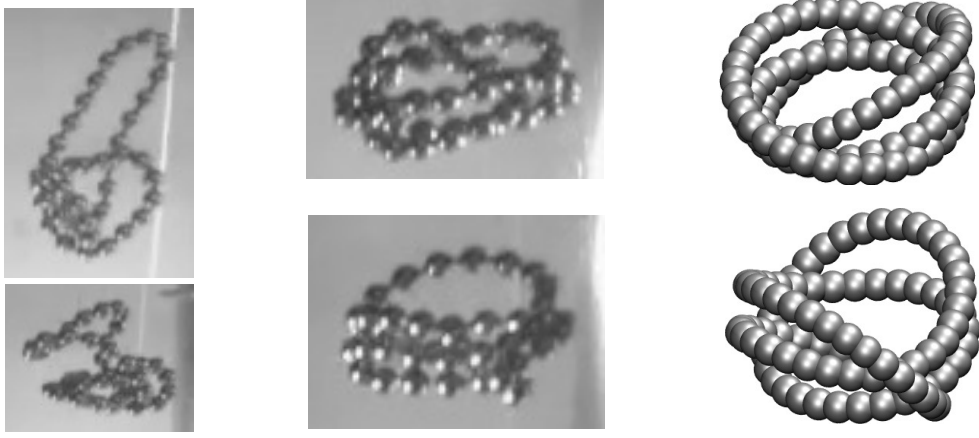

FIG. 3: Snapshots of sedimenting  $\mathcal{T}_{3,2}$  knot from experiment (initial configuration: left column, swirling: middle column) and simulation (right column,  $N = 90$ ). Gravity points downwards.

#### OTHER KNOTS: $\mathcal{T}_{2,3}$ , $\mathcal{T}_{2,5}$ , $\mathcal{T}_{2,7}$ , $\mathcal{T}_{2,9}$

Fig. 4 in the main article shows a trajectory of a bead in cylindrical coordinates  $(\tilde{\rho}, \tilde{\alpha}, \tilde{z})$  together with fitted functions (Eq. (4) in the main text). This is a trajectory from simulation of a chain of  $N=90$  beads. Below, additional plots are presented showing the limits of the approximation given by Eq. (4). Originally, this approximation has been derived in the context of a vortex of inviscid fluid in Refs. [23,24] in the main text, via perturbations of the circle and in this context should thus hold only if the deviations from the circular shape are relatively small, which corresponds to small aspect ratios (defined as the ratio of the minor to major torus radii).

In our systems, for the chains of large aspect ratios (corresponding to small  $N$ ), the elasticity comes into play. With increasing complexity of the knot (for  $q = 3, 5, 7, 9 \dots$ ) at fixed number of beads, the chain becomes more and more strained. Thus it tends to release the strain by e.g. flattening the structure (decreasing the amplitude of  $z(t)$  coordinate). Concluding, with decreasing  $N$ , although the motion (swirling) remains periodic, the approximation given in Eq. (4) in the main text begins to break, which is clearly seen in figures: Fig. 5 for  $N=40$ , Fig. 6 for  $N=60$ , and Fig. 7 for  $N=40$ . One can also see that the agreement gets worse with increasing  $q$  (compare Fig. 5 and Fig. 7 for  $N=40$ ).

On the other hand, for large enough  $N$ , higher elastic modes may appear, which is visible in Fig. 5 for  $N=120$ , in particular for  $\tilde{\rho}(t)$  (slight asymmetry of the slopes in the simulation data). At a fixed aspect ratio of the knot these modes can be damped by increasing the bending stiffness of the chain ( $A$ ). Indeed, a test simulation at 4-fold larger bending stiffness  $A' = 4A$  shows almost complete disappearance of the higher mode, see Fig. 9.

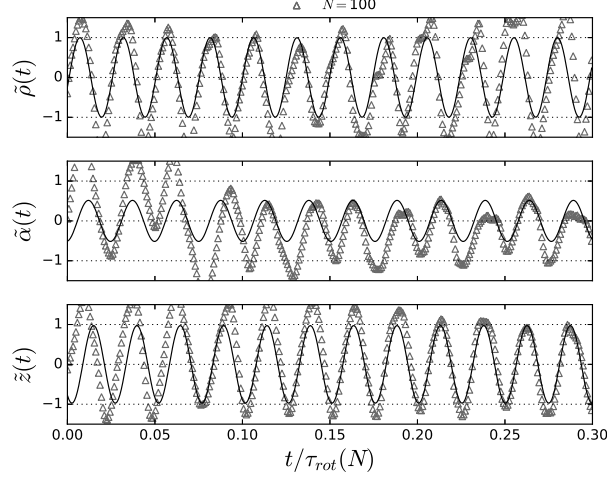

FIG. 4: Time-dependence of scaled cylindrical coordinates  $\tilde{\rho}, \tilde{\alpha}, \tilde{z}$  (see main text) of an arbitrary bead (after subtracting the constant translation and rotation), of the most long-lasting  $\mathcal{T}_{3,2}$  knot for  $N = 100$ . Simulation data (markers) and fits (lines) to Eq. (4) in the main text. Although the amplitude is irregular, a characteristic swirling frequency is visible.

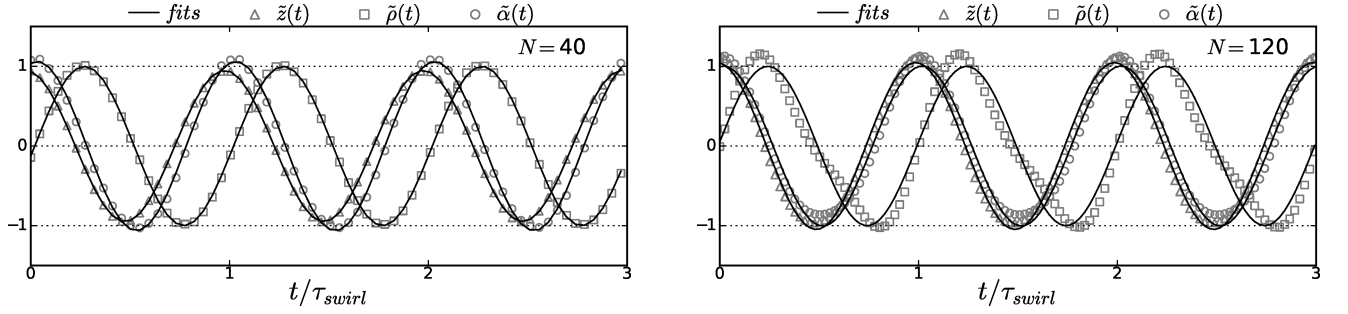

FIG. 5: Time-dependent cylindrical coordinates of the bead  $\tilde{\rho}, \tilde{\alpha}, \tilde{z}$  (after subtracting the constant translation and rotation, see Eq. (4) in the main text), in a sedimenting  $\mathcal{T}_{2,3}$  knot from simulations for  $N = 40$  (left) and  $N = 120$  (right). Simulation data (markers) and fits (lines) to the swirling motion.

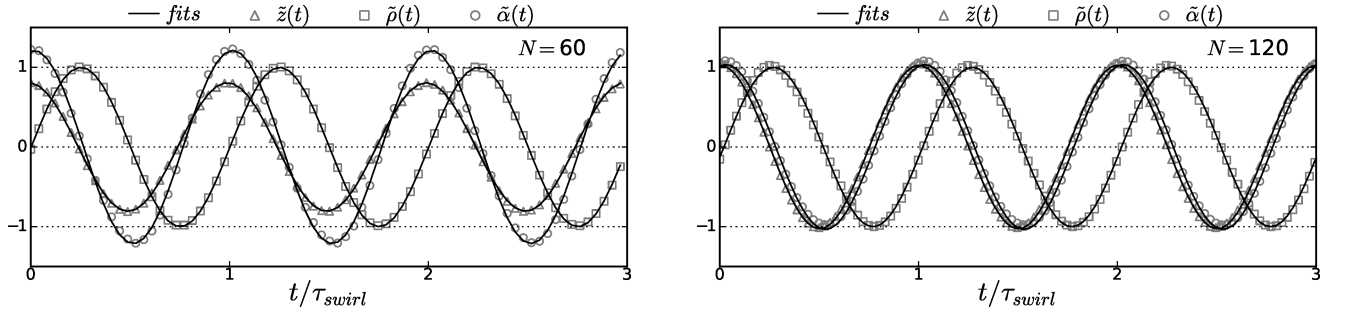

FIG. 6: As in Fig. 5 but for  $\mathcal{T}_{2,5}$  knot with  $N = 60$  (left) and  $N = 120$  (right).

This effect is even more pronounced if one plots the curvature (defined as  $\kappa = \frac{\|\mathbf{r}' \times \mathbf{r}''\|}{\|\mathbf{r}'\|^3}$ , with  $\mathbf{r} = \mathbf{r}(x(s), y(s), z(s))$ , and primes denoting derivatives over the arc length  $s$ ) along the chain length as in Fig. 10. For smaller values of  $N$  (i.e.  $N=40, 60$ , Fig. 10, left) three oscillations appear, corresponding to the lowest bending mode. On the other hand, beginning with  $N=90$  the chain becomes long enough to adopt a second bending mode (with 6 oscillations over the length of the chain).

The bending stiffness  $A$  refers to microscopic 'per angle' parameter used in the simulations, so changing the number

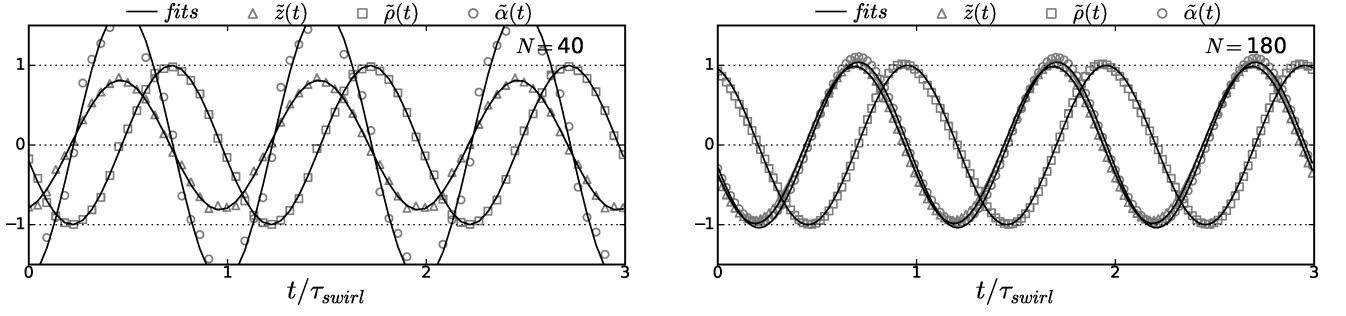

FIG. 7: As in Fig. 5 but for  $\mathcal{T}_{2,7}$  knot with  $N = 40$  (left) and  $N = 180$  (right).

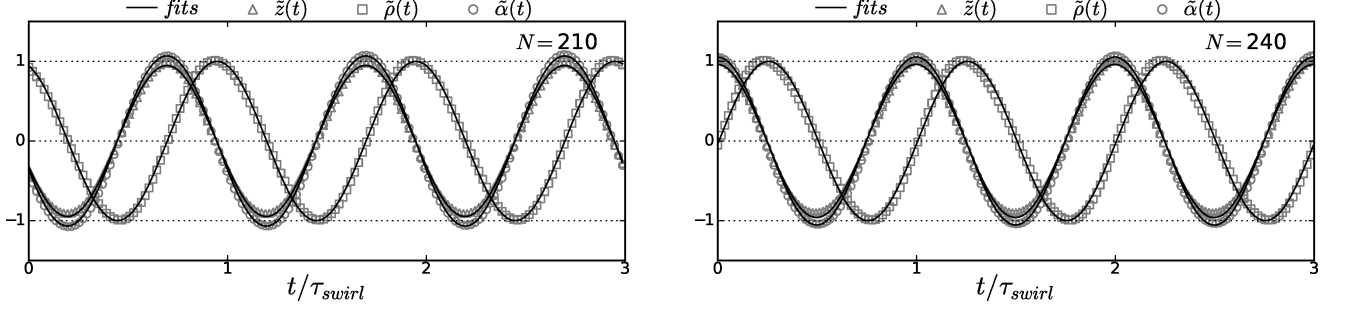

FIG. 8: As in Fig. 5 but for  $\mathcal{T}_{2,9}$  knot with  $N = 210$  (left) and  $N = 240$  (right).

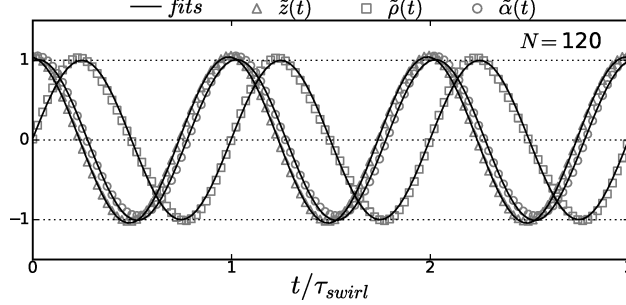

FIG. 9: As in Fig. 5 (right panel,  $N=120$ ) but for increased bending stiffness,  $A' = 4A = 20$ .

of beads ( $N$ ) and thus changing the length of the chain may be seen as decreasing the stiffness of this chain. Indeed, the results for e.g.  $N = 60, A = 5$  (Fig. 10 left, 2nd from the top) look similar to those for  $N = 120, A = 40$  (Fig. 10 right, bottom), results for  $N = 90, A = 5$  (Fig. 10 left, 3rd from the top) look similar to those for  $N = 120, A \approx 12$  (something in between  $N = 120, A = 10$  and  $N = 120, A = 20$ , Fig. 10 right, 2nd and 3rd from the top, respectively).

Systematic analysis of the dependence of the characteristic time scales on bending stiffness  $A$  is presented in Fig. 11. Clearly, the bending stiffness has much less influence on the timescales than the size  $N$  of the chains. Throughout almost 4 orders of magnitude change in  $A$ , the timescales remain within the same range. Importantly, the separation between  $\tau_{rot}$ ,  $\tau_{swirl}$  and  $\tau_{sed}$  still holds. In general, in this range of  $A$  one should expect the timescales to behave analogously to the data presented in Fig.3 in the main text.

To fill the picture, the characteristic times scales for various knot topologies, various bead numbers and for the default bending stiffness ( $A = 5$ ) are presented in Fig. 12. One can see, that both swirling and sedimentation timescales are rather not affected by the knot topologies. The rotation time does depend on the topology, but the effect of chain size (bead number) is still more pronounced. Also, the important conclusion is that the separation of timescales still holds for different topologies. For the case of  $\mathcal{T}_{3,2}$  only  $N = 100$  is presented. However, for better view, in this case  $N$  was multiplied by  $2/3$ , so that the results were overlaid onto results for the corresponding loop size. I.e. chain of  $N=60$  beads forms 2 loops of about 30 beads each in  $\mathcal{T}_{2,3}$  configuration. Chain of  $N=100$  forms 3 loops of about 33 beads each in  $\mathcal{T}_{3,2}$  configuration.

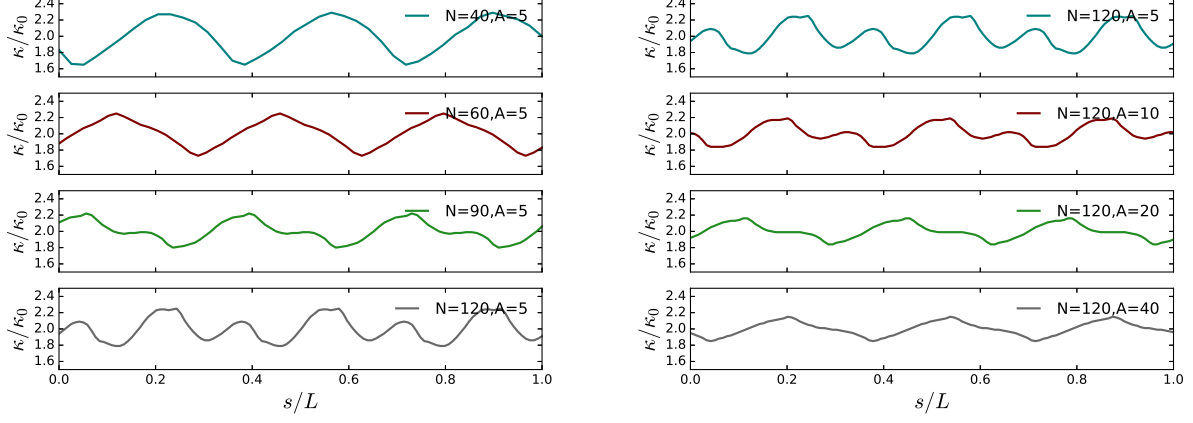

FIG. 10: Curvature along the chain for various values of  $N$  and fixed bending stiffness  $A$  (left) and for fixed  $N$  and various  $A$  (right). The arc length is normalized with its total length:  $L = \sum_1^N s_i$ , where  $s_i$  is an arc length between two consecutive beads. The curvature,  $\kappa$ , is scaled with  $\kappa_0$  that is, the curvature of the  $N$ -bead circular loop.

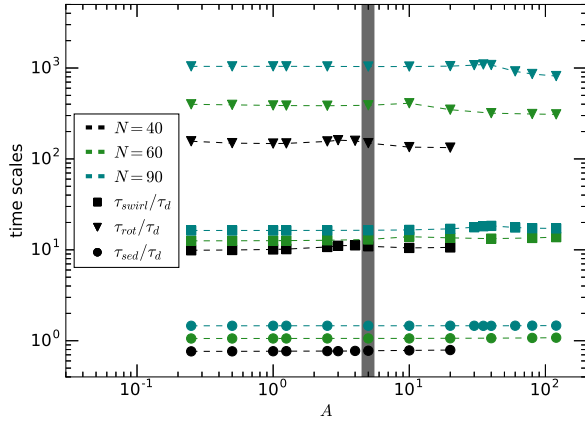

FIG. 11: Characteristic timescales practically do not depend on the bending stiffness  $A$ . Ratios of timescales obtained in simulations for swirling (squares), rotation (triangles) and sedimentation (circles) of  $\mathcal{T}_{2,3}$  loops are plotted vs the bending stiffness  $A$  for various numbers of beads in the chain,  $N=40$  (black),  $N=60$  (green), and 90 (blue). Shaded vertical region corresponds to results obtained with  $A = 5$  plotted in Fig. 3 in the main text.

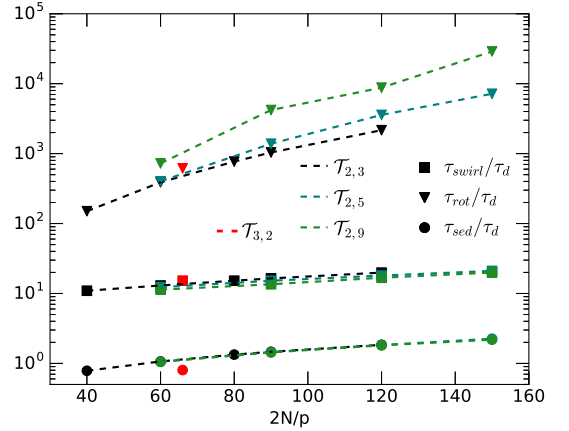

FIG. 12: Characteristic timescales for various  $\mathcal{T}_{p,q}$  knots,  $\mathcal{T}_{2,3}$  (black),  $\mathcal{T}_{2,5}$  (blue),  $\mathcal{T}_{2,9}$  (green), and  $\mathcal{T}_{3,2}$  (red) for  $A=5$ . Ratios of timescales obtained in simulations for swirling (squares), rotation (triangles) and sedimentation (circles) are plotted against number of beads in the chain. In the case of  $\mathcal{T}_{3,2}$  only  $N = 100$  is presented. However, for better view, in this case  $N$  was multiplied by  $2/3$  (to match the single loop size, see text). Black lines and markers correspond to results obtained for  $\mathcal{T}_{2,3}$  plotted in Fig. 3 in the main text.

### BEAD POSITIONS IN $z, \rho$ COORDINATES

The bead trajectories can be mapped onto 2D  $\tilde{z}-\tilde{\rho}$  (where  $\rho = (x^2 + y^2)^{1/2}$ ) plots, as presented in Figs.13-15. These sets of plots show the results for various initial knot configurations, various sizes and types of the knot. Each plot shows a single bead trajectory in scaled  $z-\rho$  coordinates (solid black line), marking its start with black cross and direction with an arrow. Additionally, the initial geometry of the torus is represented by positions of all the beads drawn as points connected with solid red lines. Also the final - stationary - geometry is drawn with solid green lines with one bead marked with a circle of the corresponding color. In the case of simulations starting from regular  $3_1$  or  $5_1$  knots (top left plots of Figs.13,14, respectively) also several intermediate geometries are shown. Again, the stationary trajectories (solid black lines in Figs.13-15) differ slightly from those that would be predicted by Eq. (4) in the main text (dashed blue lines in Figs.13-15). One should note, however, that the Eq. (4) was derived for a different system [23,24].

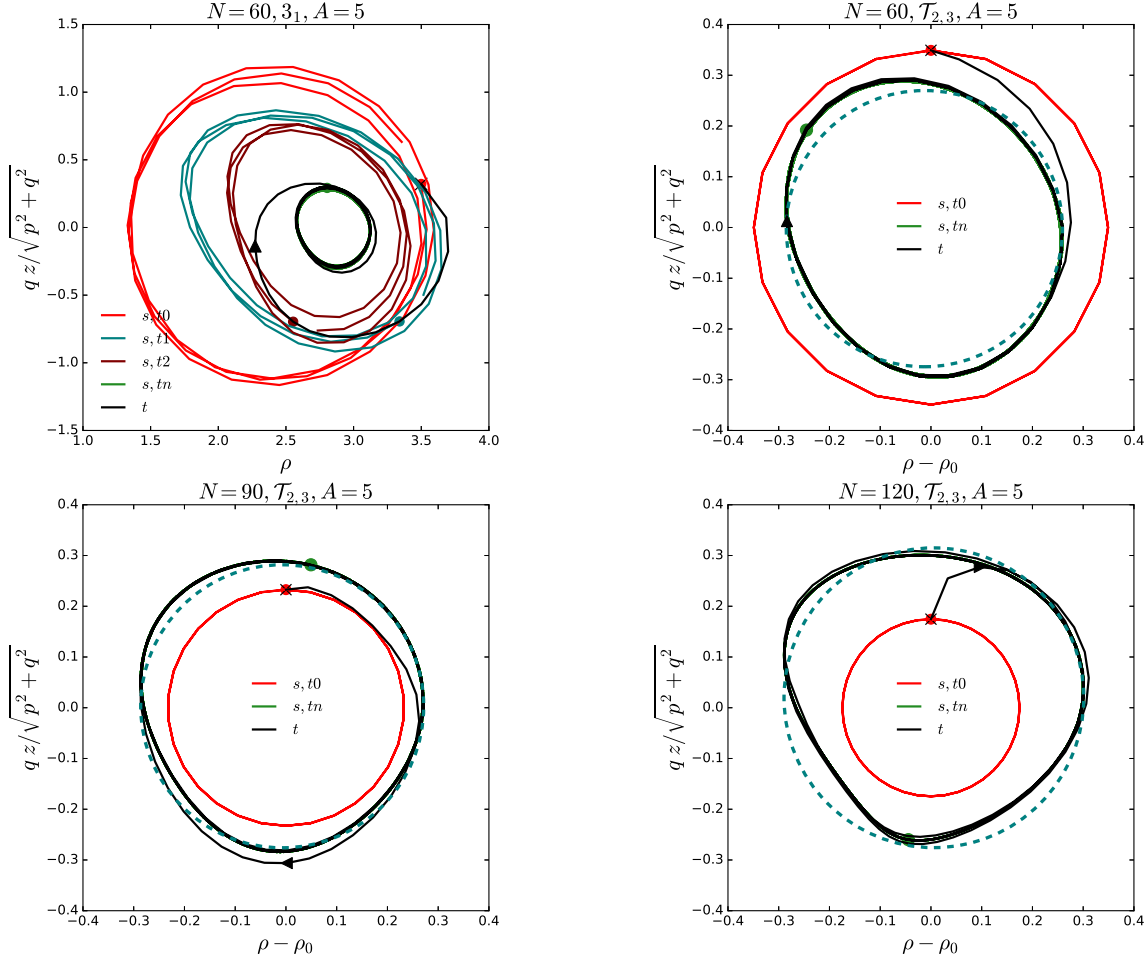

FIG. 13: Single bead trajectories (solid black lines), initial (solid red) and final (solid green) geometries of the  $3_1$  knot (top left) and  $T_{2,3}$  knot (the rest) for various chain sizes. For the case of  $3_1$  knot (top left) also several intermediate geometries at times  $t_0 < t_1 < t_2 \ll t_n$  are presented. The  $z$  coordinate is multiplied by  $q/\sqrt{p^2 + q^2}$ ; with such scaling, Eq. (4) in the main text would give circular trajectories, i.e.  $\frac{(qz)^2}{p^2 + q^2} + (\rho - \rho_0)^2 = C^2$ ; on the other hand, the scaling factor  $q/\sqrt{p^2 + q^2}$  is close to 1 (and gets even closer for higher  $q$ ) which means that also in the original (not scaled) variables the trajectories are not far from the circular shape.

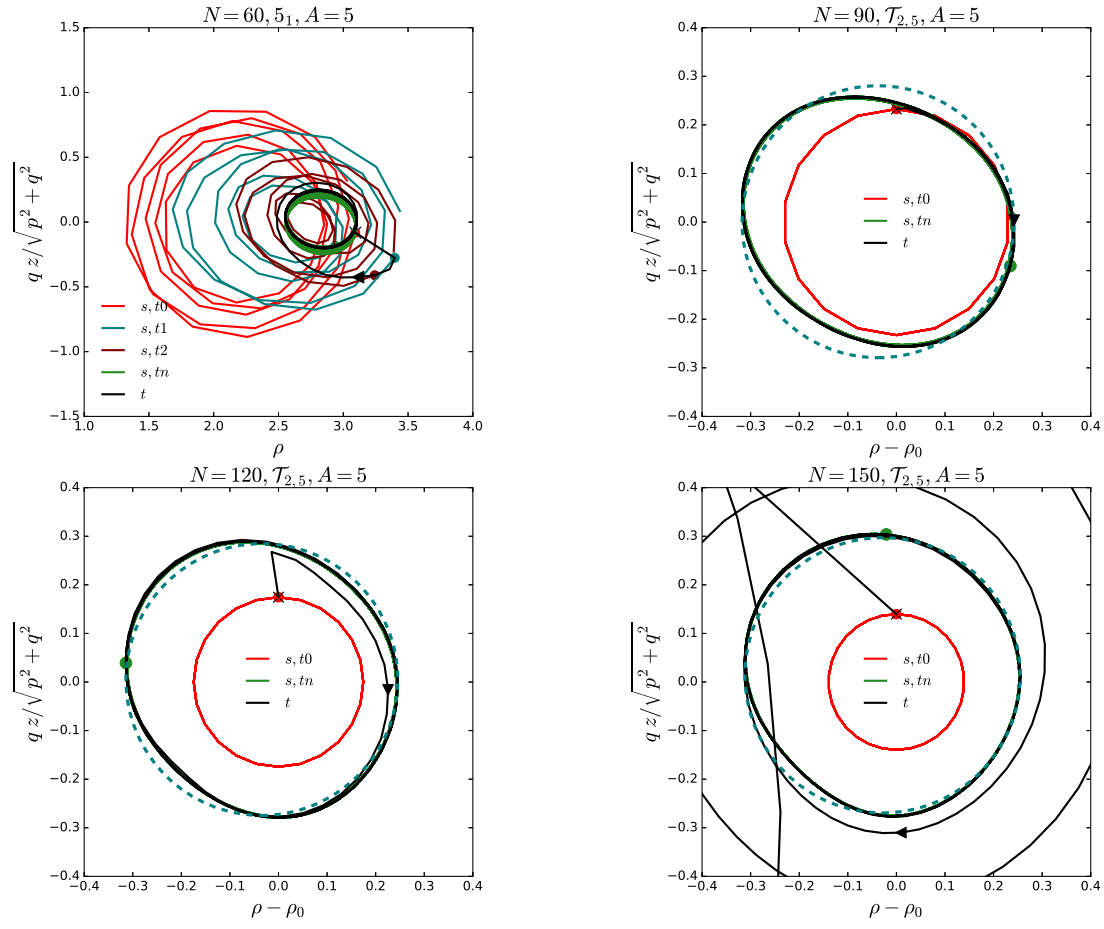FIG. 14: As in Fig.13 but for  $\mathfrak{F}_1$  and  $\mathcal{T}_{2,5}$ .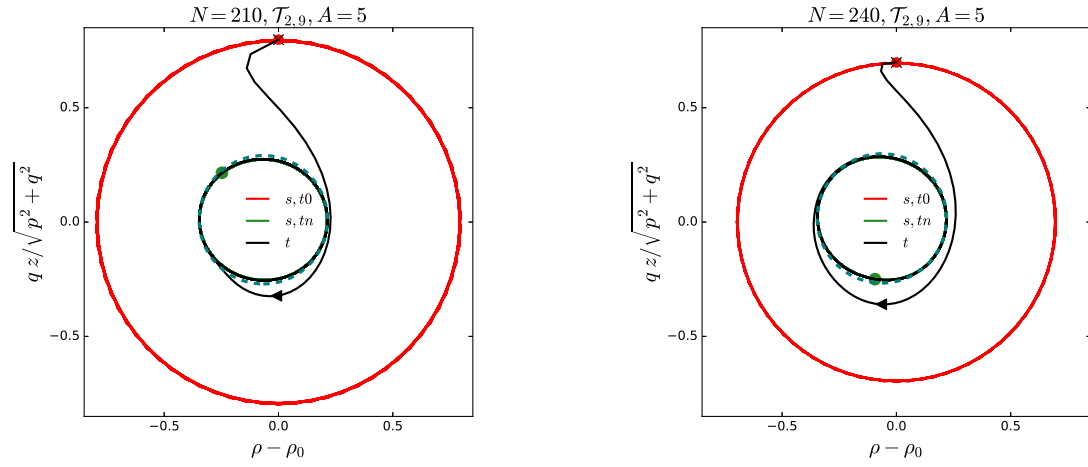FIG. 15: As in Fig.13 but for  $\mathcal{T}_{2,9}$ .

## BROWNIAN DYNAMICS

To account for Brownian motion, we perform standard Brownian dynamics simulations, with the displacements of particles given by (see e.g. [1]),

$$\Delta \mathbf{r}_i = \sum_{j=1}^N \boldsymbol{\mu}_{ij} \cdot \mathbf{F}_j \Delta t + \mathbf{R}_i, \quad (1)$$

where  $\mathbf{R}_i$  are vectors of random displacements - a Gaussian noise with zero-mean and covariance  $\langle \mathbf{R} \mathbf{R} \rangle_t = 2kT \boldsymbol{\mu} \Delta t$ . The additional drift term proportional to the divergence of the mobility matrix is omitted in Eq. 1 due to the fact that within the Rotne-Prager approximation the divergence of  $\boldsymbol{\mu}$  vanishes ( $\nabla \cdot \boldsymbol{\mu} = 0$ ). The square root of mobility matrix is obtained using Cholesky-Banachiewicz decomposition of  $\boldsymbol{\mu}$  (as described e.g. in [1]). Example simulation result is presented in the Movie 8 in this Supplementary Material. The general conclusion is that above a certain Péclet number ( $Pe \equiv \frac{dF_0}{k_B T} \geq 2$ ) the swirling motion, although less regular and with a structure flipping, is recovered, see also Fig. 16, below.

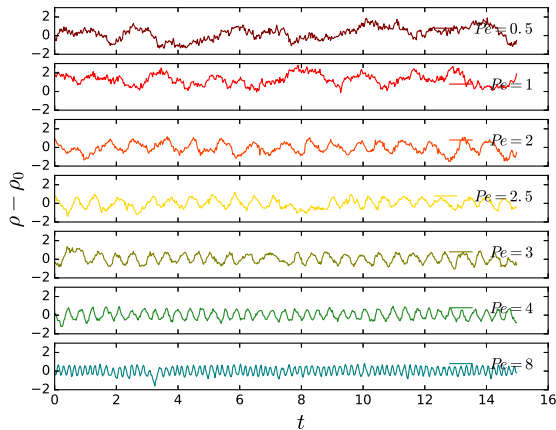

FIG. 16: Results of Brownian simulations with different values of Péclet number. Example: time dependence of the radial coordinate,  $\rho(t) - \rho_0$ , of a given bead for  $\mathcal{T}_{2,3}$  knot with  $N=40$  beads, and with Brownian motion present. Péclet numbers are given in plot legends.

---

[1] M. P. Allen and D. J. Tildesley, *Computer Simulation of Liquids*, 2nd ed., edited by O. U. Press (2017).
